# Supplementary material for: Cost-Efficient Subjective Task Annotation and Modeling through Few-Shot Annotator Adaptation
Source: arXiv:2402.14101 source file (2024-09-05)
Supplement: Supplementary file 1 [file 8.appendix_mfrc.tex]

\section{MFRC results}

\begin{table} \small
\caption{Results for mtl 24 with 0.25 budget (train size : 400) on mfrc dataset}
\begin{tabular}{l|cc}
\toprule
Annotator & F1 & AUC \\
 \hline \midrule
0 & 0.898734 & 0.827526 \\
1 & 0.850000 & 0.736264 \\
2 & 0.804688 & 0.709821 \\
3 & 0.781250 & 0.705741 \\
4 & 0.846154 & 0.707182 \\
5 & 0.761905 & 0.689978 \\
6 & 0.704000 & 0.630000 \\
7 & 0.850174 & 0.723033 \\
8 & 0.878049 & 0.777235 \\
9 & 0.800000 & 0.659915 \\
10 & 0.746781 & 0.712065 \\
11 & 0.714894 & 0.695579 \\
12 & 0.790698 & 0.689827 \\
13 & 0.877743 & 0.747535 \\
14 & 0.572770 & 0.659309 \\
15 & 0.438503 & 0.641429 \\
16 & 0.446701 & 0.621680 \\
17 & 0.774468 & 0.683395 \\
18 & 0.885350 & 0.778050 \\
19 & 0.819923 & 0.736299 \\
20 & 0.830189 & 0.728922 \\
21 & 0.853659 & 0.665986 \\
22 & 0.880952 & 0.826421 \\
23 & 0.643478 & 0.638994 \\
Overall & 0.768794 & 0.708008 \\
\bottomrule
\end{tabular}
\end{table}

\begin{table} \small
\caption{Results for mtl 24 with 0.5 budget (train size: 800) on mfrc dataset}
\begin{tabular}{l|cc}
\toprule
Annotator & F1 & AUC \\
 \hline \midrule
0 & 0.921136 & 0.894916 \\
1 & 0.854093 & 0.740110 \\
2 & 0.840467 & 0.756533 \\
3 & 0.785992 & 0.710458 \\
4 & 0.864111 & 0.735517 \\
5 & 0.766798 & 0.694832 \\
6 & 0.733068 & 0.665000 \\
7 & 0.875000 & 0.761441 \\
8 & 0.899696 & 0.863408 \\
9 & 0.804428 & 0.663883 \\
10 & 0.743590 & 0.707211 \\
11 & 0.717949 & 0.700084 \\
12 & 0.810811 & 0.715368 \\
13 & 0.887500 & 0.770118 \\
14 & 0.579439 & 0.667246 \\
15 & 0.444444 & 0.650000 \\
16 & 0.454545 & 0.632318 \\
17 & 0.774468 & 0.683395 \\
18 & 0.901587 & 0.818336 \\
19 & 0.839695 & 0.761186 \\
20 & 0.857143 & 0.765102 \\
21 & 0.863222 & 0.694331 \\
22 & 0.896142 & 0.905914 \\
23 & 0.658009 & 0.655576 \\
Overall & 0.782222 & 0.733845 \\
\bottomrule
\end{tabular}
\end{table}

\begin{table} \small
\caption{Results for mtl 24 with 0.75 budget (train size : 1200) on mfrc dataset}
\begin{tabular}{l|cc}
\toprule
Annotator & F1 & AUC \\
 \hline \midrule
0 & 0.885246 & 0.880890 \\
1 & 0.855019 & 0.770879 \\
2 & 0.840816 & 0.776895 \\
3 & 0.800000 & 0.744179 \\
4 & 0.843636 & 0.741828 \\
5 & 0.780083 & 0.727144 \\
6 & 0.736402 & 0.685000 \\
7 & 0.876812 & 0.798749 \\
8 & 0.864353 & 0.857682 \\
9 & 0.826255 & 0.730573 \\
10 & 0.783784 & 0.765463 \\
11 & 0.756757 & 0.754138 \\
12 & 0.825911 & 0.755303 \\
13 & 0.870130 & 0.813116 \\
14 & 0.613861 & 0.711042 \\
15 & 0.451977 & 0.659524 \\
16 & 0.483871 & 0.671534 \\
17 & 0.791111 & 0.722778 \\
18 & 0.877888 & 0.838102 \\
19 & 0.848000 & 0.789306 \\
20 & 0.842520 & 0.767492 \\
21 & 0.820189 & 0.660623 \\
22 & 0.855385 & 0.873656 \\
23 & 0.684932 & 0.696014 \\
Overall & 0.783956 & 0.757996 \\
\bottomrule
\end{tabular}
\end{table}

\begin{table} \small
\caption{Results for mtl 24 with 1.0 budget (train size : 1600) on mfrc dataset}
\begin{tabular}{l|cc}
\toprule
Annotator & F1 & AUC \\
 \hline \midrule
0 & 0.831615 & 0.839470 \\
1 & 0.828125 & 0.764835 \\
2 & 0.836207 & 0.792792 \\
3 & 0.827586 & 0.793256 \\
4 & 0.832061 & 0.769279 \\
5 & 0.771930 & 0.734476 \\
6 & 0.707965 & 0.670000 \\
7 & 0.844106 & 0.786062 \\
8 & 0.815789 & 0.821369 \\
9 & 0.809717 & 0.740109 \\
10 & 0.800000 & 0.792298 \\
11 & 0.777251 & 0.783050 \\
12 & 0.829060 & 0.780195 \\
13 & 0.820339 & 0.774655 \\
14 & 0.645503 & 0.746901 \\
15 & 0.475610 & 0.687619 \\
16 & 0.508671 & 0.700111 \\
17 & 0.792453 & 0.747160 \\
18 & 0.838488 & 0.820595 \\
19 & 0.869198 & 0.833385 \\
20 & 0.863071 & 0.818883 \\
21 & 0.789474 & 0.700715 \\
22 & 0.807692 & 0.838710 \\
23 & 0.679612 & 0.699048 \\
Overall & 0.775063 & 0.768124 \\
\bottomrule
\end{tabular}
\end{table}

\begin{table*} \small
\caption{Results Few shot on 6 mtl mfrc, selection method : balanced mv}
\label{tab:mfrc}
\begin{tabular}{l|cccc}
\toprule
Annotator & 16 & 32 & 64 & 128 \\
\hline \midrule
0 & 0.934 (0.007) / 0.674 (0.057) & 0.932 (0.008) / 0.638 (0.066) & 0.934 (0.006) / 0.651 (0.069) & 0.933 (0.005) / 0.621 (0.068) \\
1 & 0.845 (0.016) / 0.723 (0.066) & 0.855 (0.012) / 0.753 (0.036) & 0.853 (0.015) / 0.748 (0.038) & 0.852 (0.016) / 0.76 (0.028) \\
10 & 0.732 (0.04) / 0.756 (0.023) & 0.749 (0.042) / 0.766 (0.025) & 0.756 (0.029) / 0.77 (0.022) & 0.765 (0.035) / 0.782 (0.024) \\
11 & 0.741 (0.029) / 0.761 (0.03) & 0.743 (0.032) / 0.766 (0.026) & 0.749 (0.028) / 0.773 (0.026) & 0.75 (0.025) / 0.775 (0.022) \\
12 & 0.805 (0.023) / 0.745 (0.05) & 0.801 (0.031) / 0.749 (0.065) & 0.81 (0.024) / 0.763 (0.033) & 0.816 (0.031) / 0.773 (0.038) \\
13 & 0.918 (0.004) / 0.547 (0.052) & 0.917 (0.006) / 0.549 (0.064) & 0.919 (0.006) / 0.541 (0.042) & 0.918 (0.004) / 0.531 (0.037) \\
14 & 0.63 (0.042) / 0.731 (0.03) & 0.636 (0.039) / 0.736 (0.026) & 0.644 (0.051) / 0.742 (0.034) & 0.643 (0.038) / 0.74 (0.028) \\
15 & 0.539 (0.036) / 0.71 (0.023) & 0.553 (0.047) / 0.725 (0.032) & 0.551 (0.045) / 0.719 (0.032) & 0.587 (0.041) / 0.741 (0.025) \\
16 & 0.512 (0.041) / 0.689 (0.037) & 0.527 (0.033) / 0.7 (0.029) & 0.517 (0.042) / 0.689 (0.035) & 0.532 (0.056) / 0.7 (0.042) \\
17 & 0.763 (0.02) / 0.722 (0.017) & 0.768 (0.02) / 0.727 (0.021) & 0.766 (0.012) / 0.721 (0.014) & 0.762 (0.019) / 0.724 (0.02) \\
18 & 0.915 (0.016) / 0.654 (0.109) & 0.92 (0.009) / 0.644 (0.082) & 0.925 (0.007) / 0.671 (0.065) & 0.924 (0.008) / 0.644 (0.073) \\
19 & 0.835 (0.023) / 0.796 (0.031) & 0.846 (0.015) / 0.811 (0.018) & 0.847 (0.014) / 0.808 (0.014) & 0.846 (0.016) / 0.808 (0.02) \\
2 & 0.827 (0.013) / 0.775 (0.027) & 0.827 (0.02) / 0.783 (0.024) & 0.829 (0.015) / 0.785 (0.027) & 0.832 (0.017) / 0.784 (0.024) \\
20 & 0.833 (0.03) / 0.784 (0.037) & 0.833 (0.024) / 0.789 (0.019) & 0.833 (0.035) / 0.79 (0.024) & 0.843 (0.018) / 0.794 (0.025) \\
21 & 0.938 (0.009) / 0.601 (0.082) & 0.941 (0.007) / 0.608 (0.081) & 0.936 (0.012) / 0.646 (0.076) & 0.936 (0.016) / 0.629 (0.089) \\
22 & 0.964 (0.006) / 0.554 (0.043) & 0.963 (0.007) / 0.573 (0.059) & 0.965 (0.003) / 0.575 (0.058) & 0.966 (0.003) / 0.557 (0.036) \\
23 & 0.662 (0.037) / 0.711 (0.026) & 0.648 (0.042) / 0.702 (0.036) & 0.671 (0.037) / 0.723 (0.023) & 0.679 (0.028) / 0.721 (0.037) \\
3 & 0.795 (0.012) / 0.768 (0.021) & 0.793 (0.033) / 0.77 (0.026) & 0.794 (0.015) / 0.77 (0.013) & 0.799 (0.018) / 0.778 (0.018) \\
4 & 0.845 (0.01) / 0.701 (0.034) & 0.839 (0.009) / 0.687 (0.042) & 0.845 (0.009) / 0.699 (0.019) & 0.843 (0.01) / 0.682 (0.033) \\
5 & 0.758 (0.018) / 0.7 (0.035) & 0.762 (0.018) / 0.708 (0.035) & 0.763 (0.014) / 0.712 (0.024) & 0.768 (0.017) / 0.731 (0.02) \\
6 & 0.718 (0.017) / 0.692 (0.016) & 0.726 (0.017) / 0.694 (0.017) & 0.712 (0.02) / 0.689 (0.015) & 0.714 (0.011) / 0.692 (0.015) \\
7 & 0.852 (0.01) / 0.749 (0.043) & 0.85 (0.009) / 0.741 (0.042) & 0.848 (0.011) / 0.737 (0.032) & 0.851 (0.016) / 0.747 (0.042) \\
8 & 0.941 (0.005) / 0.559 (0.082) & 0.941 (0.005) / 0.58 (0.084) & 0.941 (0.006) / 0.56 (0.072) & 0.944 (0.004) / 0.525 (0.044) \\
9 & 0.807 (0.01) / 0.704 (0.031) & 0.806 (0.014) / 0.705 (0.025) & 0.805 (0.013) / 0.692 (0.035) & 0.805 (0.013) / 0.691 (0.026) \\
\hline Total & 0.796 (0.121) / 0.7 (0.071) & 0.799 (0.118) / 0.704 (0.072) & 0.801 (0.119) / 0.707 (0.072) & 0.805 (0.113) / 0.705 (0.082) \\
\bottomrule
\end{tabular}
\end{table*}

\begin{table*} \small
\caption{Results Few shot on 12 mtl mfrc, selection method : balanced mv}
\label{tab:mfrc}
\begin{tabular}{l|cccc}
\toprule
Annotator & 16 & 32 & 64 & 128 \\
\hline \midrule
0 & 0.933 (0.009) / 0.663 (0.139) & 0.934 (0.005) / 0.632 (0.079) & 0.933 (0.008) / 0.604 (0.072) & 0.932 (0.007) / 0.596 (0.075) \\
1 & 0.853 (0.012) / 0.764 (0.021) & 0.856 (0.01) / 0.768 (0.035) & 0.852 (0.013) / 0.762 (0.033) & 0.854 (0.017) / 0.772 (0.037) \\
10 & 0.755 (0.048) / 0.752 (0.091) & 0.767 (0.05) / 0.765 (0.094) & 0.765 (0.049) / 0.764 (0.094) & 0.744 (0.042) / 0.751 (0.089) \\
11 & 0.737 (0.059) / 0.753 (0.068) & 0.727 (0.044) / 0.741 (0.08) & 0.734 (0.047) / 0.748 (0.083) & 0.743 (0.046) / 0.764 (0.054) \\
12 & 0.797 (0.03) / 0.716 (0.082) & 0.804 (0.033) / 0.739 (0.087) & 0.802 (0.035) / 0.74 (0.087) & 0.807 (0.035) / 0.744 (0.089) \\
13 & 0.917 (0.004) / 0.527 (0.03) & 0.916 (0.008) / 0.545 (0.043) & 0.918 (0.003) / 0.542 (0.039) & 0.919 (0.002) / 0.523 (0.034) \\
14 & 0.662 (0.032) / 0.756 (0.025) & 0.645 (0.039) / 0.742 (0.028) & 0.648 (0.043) / 0.745 (0.03) & 0.643 (0.04) / 0.74 (0.028) \\
15 & 0.537 (0.062) / 0.711 (0.037) & 0.537 (0.049) / 0.71 (0.032) & 0.538 (0.052) / 0.711 (0.034) & 0.567 (0.063) / 0.725 (0.039) \\
16 & 0.532 (0.032) / 0.703 (0.021) & 0.544 (0.037) / 0.714 (0.031) & 0.547 (0.027) / 0.711 (0.02) & 0.556 (0.034) / 0.718 (0.019) \\
17 & 0.759 (0.026) / 0.697 (0.088) & 0.756 (0.03) / 0.689 (0.085) & 0.762 (0.033) / 0.7 (0.089) & 0.757 (0.027) / 0.693 (0.081) \\
18 & 0.921 (0.009) / 0.663 (0.094) & 0.92 (0.01) / 0.631 (0.082) & 0.92 (0.009) / 0.656 (0.093) & 0.925 (0.008) / 0.646 (0.076) \\
19 & 0.85 (0.011) / 0.807 (0.021) & 0.85 (0.011) / 0.811 (0.015) & 0.851 (0.015) / 0.817 (0.018) & 0.857 (0.011) / 0.816 (0.017) \\
2 & 0.828 (0.017) / 0.767 (0.028) & 0.828 (0.013) / 0.777 (0.025) & 0.835 (0.018) / 0.783 (0.019) & 0.835 (0.019) / 0.794 (0.017) \\
20 & 0.835 (0.039) / 0.769 (0.096) & 0.841 (0.037) / 0.779 (0.099) & 0.846 (0.034) / 0.777 (0.098) & 0.842 (0.031) / 0.791 (0.047) \\
21 & 0.937 (0.017) / 0.605 (0.072) & 0.938 (0.012) / 0.598 (0.071) & 0.935 (0.013) / 0.628 (0.086) & 0.94 (0.01) / 0.628 (0.084) \\
22 & 0.965 (0.003) / 0.568 (0.034) & 0.966 (0.003) / 0.577 (0.053) & 0.964 (0.002) / 0.555 (0.046) & 0.966 (0.003) / 0.56 (0.046) \\
23 & 0.667 (0.039) / 0.689 (0.069) & 0.658 (0.04) / 0.692 (0.069) & 0.663 (0.037) / 0.697 (0.071) & 0.665 (0.036) / 0.703 (0.072) \\
3 & 0.817 (0.009) / 0.786 (0.013) & 0.807 (0.016) / 0.786 (0.012) & 0.802 (0.018) / 0.774 (0.025) & 0.795 (0.012) / 0.78 (0.009) \\
4 & 0.84 (0.014) / 0.685 (0.025) & 0.835 (0.019) / 0.672 (0.05) & 0.841 (0.023) / 0.687 (0.055) & 0.847 (0.008) / 0.688 (0.025) \\
5 & 0.757 (0.02) / 0.71 (0.027) & 0.765 (0.014) / 0.716 (0.03) & 0.763 (0.02) / 0.722 (0.024) & 0.766 (0.01) / 0.715 (0.017) \\
6 & 0.739 (0.01) / 0.708 (0.009) & 0.729 (0.011) / 0.695 (0.018) & 0.73 (0.013) / 0.696 (0.017) & 0.725 (0.016) / 0.702 (0.015) \\
7 & 0.853 (0.019) / 0.729 (0.09) & 0.855 (0.018) / 0.728 (0.093) & 0.854 (0.019) / 0.717 (0.085) & 0.855 (0.019) / 0.714 (0.052) \\
8 & 0.94 (0.008) / 0.59 (0.097) & 0.942 (0.006) / 0.549 (0.071) & 0.941 (0.006) / 0.575 (0.108) & 0.942 (0.004) / 0.536 (0.068) \\
9 & 0.808 (0.013) / 0.681 (0.064) & 0.806 (0.013) / 0.681 (0.064) & 0.808 (0.013) / 0.68 (0.061) & 0.809 (0.01) / 0.692 (0.027) \\
\hline Total & 0.802 (0.117) / 0.7 (0.071) & 0.801 (0.118) / 0.697 (0.075) & 0.802 (0.117) / 0.7 (0.074) & 0.804 (0.114) / 0.7 (0.081) \\
\bottomrule
\end{tabular}
\end{table*}

\begin{table*} \small
\caption{Results Few shot on 18 mtl mfrc, selection method : balanced mv}
\label{tab:mfrc}
\begin{tabular}{l|cccc}
\toprule
Annotator & 16 & 32 & 64 & 128 \\
\hline \midrule
0 & 0.932 (0.004) / 0.613 (0.068) & 0.933 (0.001) / 0.592 (0.024) & 0.929 (0.001) / 0.535 (0.017) & 0.933 (0.004) / 0.581 (0.05) \\
1 & 0.849 (0.013) / 0.764 (0.032) & 0.851 (0.018) / 0.773 (0.027) & 0.859 (0.008) / 0.779 (0.029) & 0.862 (0.013) / 0.778 (0.034) \\
10 & 0.762 (0.058) / 0.781 (0.028) & 0.775 (0.036) / 0.79 (0.023) & 0.779 (0.017) / 0.79 (0.01) & 0.761 (0.037) / 0.783 (0.024) \\
11 & 0.767 (0.018) / 0.786 (0.015) & 0.762 (0.021) / 0.783 (0.013) & 0.745 (0.045) / 0.774 (0.03) & 0.758 (0.027) / 0.784 (0.019) \\
12 & 0.814 (0.024) / 0.734 (0.059) & 0.817 (0.016) / 0.752 (0.046) & 0.831 (0.011) / 0.778 (0.022) & 0.843 (0.007) / 0.798 (0.008) \\
13 & 0.918 (0.005) / 0.527 (0.03) & 0.92 (0.002) / 0.529 (0.037) & 0.919 (0.002) / 0.545 (0.042) & 0.92 (0.002) / 0.554 (0.075) \\
14 & 0.645 (0.037) / 0.743 (0.027) & 0.65 (0.024) / 0.745 (0.019) & 0.663 (0.029) / 0.755 (0.022) & 0.638 (0.063) / 0.739 (0.042) \\
15 & 0.54 (0.006) / 0.716 (0.004) & 0.542 (0.022) / 0.717 (0.016) & 0.582 (0.019) / 0.74 (0.022) & 0.577 (0.025) / 0.745 (0.015) \\
16 & 0.501 (0.02) / 0.676 (0.01) & 0.518 (0.011) / 0.688 (0.007) & 0.506 (0.009) / 0.68 (0.012) & 0.531 (0.001) / 0.698 (0.005) \\
17 & 0.774 (0.02) / 0.716 (0.0) & 0.771 (0.013) / 0.714 (0.001) & 0.769 (0.016) / 0.711 (0.003) & 0.752 (0.013) / 0.724 (0.001) \\
18 & 0.923 (0.003) / 0.72 (0.071) & 0.92 (0.002) / 0.756 (0.002) & 0.917 (0.01) / 0.786 (0.018) & 0.927 (0.002) / 0.698 (0.076) \\
19 & 0.858 (0.017) / 0.809 (0.028) & 0.857 (0.013) / 0.806 (0.02) & 0.855 (0.007) / 0.81 (0.014) & 0.855 (0.012) / 0.824 (0.011) \\
2 & 0.832 (0.022) / 0.772 (0.03) & 0.85 (0.015) / 0.8 (0.022) & 0.843 (0.016) / 0.785 (0.024) & 0.839 (0.013) / 0.787 (0.01) \\
20 & 0.846 (0.014) / 0.814 (0.011) & 0.84 (0.026) / 0.815 (0.014) & 0.846 (0.017) / 0.804 (0.009) & 0.859 (0.012) / 0.819 (0.014) \\
21 & 0.945 (0.004) / 0.629 (0.063) & 0.941 (0.013) / 0.617 (0.039) & 0.944 (0.003) / 0.555 (0.043) & 0.951 (0.004) / 0.634 (0.071) \\
22 & 0.965 (0.003) / 0.551 (0.021) & 0.964 (0.003) / 0.55 (0.022) & 0.965 (0.003) / 0.552 (0.02) & 0.967 (0.001) / 0.553 (0.034) \\
23 & 0.659 (0.032) / 0.7 (0.037) & 0.656 (0.04) / 0.704 (0.035) & 0.68 (0.037) / 0.729 (0.029) & 0.695 (0.003) / 0.738 (0.005) \\
3 & 0.805 (0.018) / 0.782 (0.016) & 0.81 (0.02) / 0.786 (0.016) & 0.805 (0.016) / 0.781 (0.018) & 0.806 (0.009) / 0.781 (0.009) \\
4 & 0.849 (0.014) / 0.718 (0.035) & 0.848 (0.011) / 0.728 (0.019) & 0.842 (0.013) / 0.685 (0.058) & 0.843 (0.009) / 0.698 (0.033) \\
5 & 0.77 (0.013) / 0.711 (0.024) & 0.77 (0.008) / 0.719 (0.022) & 0.766 (0.015) / 0.72 (0.019) & 0.759 (0.009) / 0.728 (0.013) \\
6 & 0.72 (0.02) / 0.685 (0.014) & 0.723 (0.029) / 0.698 (0.039) & 0.707 (0.056) / 0.665 (0.085) & 0.707 (0.039) / 0.688 (0.032) \\
7 & 0.855 (0.004) / 0.762 (0.017) & 0.861 (0.006) / 0.755 (0.027) & 0.857 (0.006) / 0.741 (0.025) & 0.859 (0.006) / 0.745 (0.023) \\
8 & 0.943 (0.003) / 0.518 (0.029) & 0.944 (0.004) / 0.511 (0.013) & 0.945 (0.001) / 0.507 (0.013) & 0.946 (0.003) / 0.544 (0.056) \\
9 & 0.803 (0.016) / 0.691 (0.055) & 0.819 (0.007) / 0.71 (0.028) & 0.828 (0.001) / 0.727 (0.02) & 0.826 (0.007) / 0.714 (0.003) \\
\hline Total & 0.803 (0.122) / 0.705 (0.084) & 0.806 (0.12) / 0.71 (0.088) & 0.808 (0.116) / 0.706 (0.096) & 0.809 (0.117) / 0.714 (0.084) \\
\bottomrule
\end{tabular}
\end{table*}
